# Supplementary material for: Adaptive cluster approximation for reduced density-matrix functional theory
Source: arXiv:1612.06692 ancillary file (2018-05-16)
Supplement: Supplementary file 1 [file supp.pdf]

# Supplemental Material: Adaptive cluster approximation for reduced density-matrix functional theory

Robert Schade[1,*] and Peter E. Blöchl[1,2]

[1]Institute for Theoretical Physics, Clausthal University of Technology, Leibnizstr. 10, 38678 Clausthal-Zellerfeld, Germany

[2]Institute for Materials Physics, Georg-August-Universität Göttingen, Friedrich-Hund-Platz 1, 37077 Göttingen, Germany

(Dated: May 16, 2018)

## CONTENTS

I. Invariance of the density-matrix functional 1

II. Practical construction of the transformation 2
A. One unitary transformation step 2
B. Iterated transformations 2

III. Exact decoupling 3

IV. Evaluation of the exact density-matrix functional 4

V. SIAM in additional parameter regimes 5
A. Impurity on-site-energy dependence 5
1. Exact results 5
2. ACA results 6
B. Bandwidth dependence 7
1. Exact results 7
2. ACA results 8

References 8

## I. INVARIANCE OF THE DENSITY-MATRIX FUNCTIONAL

Here we prove the invariance of the density-matrix functional with respect to transformations of the one-particle reduced density matrix, Eq. 13 of the paper,

$$F^{\hat{W}}_{\beta}[\boldsymbol{\rho}] = F^{\hat{W}}_{\beta}[\boldsymbol{U}^{\dagger}\boldsymbol{\rho}\boldsymbol{U}], \tag{S1}$$

with a $N_{\chi} \times N_{\chi}$ unitary matrix of the form

$$\boldsymbol{U} = \begin{pmatrix} \boldsymbol{1}_{N_{\rm imp}} & \boldsymbol{0} \\ \boldsymbol{0} & \boldsymbol{U}^{\dagger}_{\rm bath} \end{pmatrix}. \tag{S2}$$

This transform does not act on interacting orbitals.

With the density-matrix functional written as the Legendre-Fenchel transform of the grand potential with respect to the one-particle Hamiltonian, we obtain

$$F^{\hat{W}}_{\beta}[\boldsymbol{U}^{\dagger}\boldsymbol{\rho}\boldsymbol{U}] = \max_{\boldsymbol{h},\mu} \left[\Omega^{\hat{W}}_{\beta,\mu}[\boldsymbol{h}] - {\rm Tr}(\boldsymbol{U}^{\dagger}\boldsymbol{\rho}\boldsymbol{U}\boldsymbol{h})\right] \tag{S3}$$

$$= \max_{\boldsymbol{h},\mu} \left[\Omega^{\hat{W}}_{\beta,\mu}[\boldsymbol{h}] - {\rm Tr}(\boldsymbol{\rho}\boldsymbol{U}\boldsymbol{h}\boldsymbol{U}^{\dagger})\right]. \tag{S4}$$

Next we define the transformed matrix elements $\tilde{\boldsymbol{h}} = \boldsymbol{U}\boldsymbol{h}\boldsymbol{U}^{\dagger}$ of the one-particle Hamiltonian and write the above maximization over these matrix elements as

$$F^{\hat{W}}_{\beta}[\boldsymbol{U}^{\dagger}\boldsymbol{\rho}\boldsymbol{U}] = \max_{\tilde{\boldsymbol{h}},\mu} \left[\Omega^{\hat{W}}_{\beta,\mu}[\boldsymbol{U}^{\dagger}\tilde{\boldsymbol{h}}\boldsymbol{U}] - {\rm Tr}(\boldsymbol{\rho}\tilde{\boldsymbol{h}})\right]. \tag{S5}$$

For the grand potential $\Omega^{\hat{W}}_{\beta,\mu}[\boldsymbol{U}^{\dagger}\tilde{\boldsymbol{h}}\boldsymbol{U}]$ we now use its definition Eq. (A2) to obtain

$$\Omega^{\hat{W}}_{\beta,\mu}[\boldsymbol{U}^{\dagger}\tilde{\boldsymbol{h}}\boldsymbol{U}] = -\frac{1}{\beta}\ln\left({\rm Tr}e^{-\beta(\hat{W}-\mu\hat{N}+\sum_{i,j}(\boldsymbol{U}^{\dagger}\tilde{\boldsymbol{h}}\boldsymbol{U})_{i,j}\hat{c}^{\dagger}_i\hat{c}_j)}\right). \tag{S6}$$

Next we introduce transformed creation $\hat{\tilde{c}}^{\dagger}_a$ and annihilation operators $\hat{\tilde{c}}^{\dagger}_a$ given by

$$\hat{\tilde{c}}^{\dagger}_a = \sum_i U^{*}_{a,i}\hat{c}^{\dagger}_i \tag{S7}$$

$$\hat{\tilde{c}}_b = \sum_i U_{b,i}\hat{c}_i. \tag{S8}$$

Because $\boldsymbol{U}$ does not act on the interacting states, Eq. (S2), the interaction remains unchanged

$$\hat{W} = \sum_{abcd} W_{abcd}\hat{c}^{\dagger}_a\hat{c}^{\dagger}_b\hat{c}_d\hat{c}_c \tag{S9}$$

$$= \sum_{abcd} W_{abcd}\hat{\tilde{c}}^{\dagger}_a\hat{\tilde{c}}^{\dagger}_b\hat{\tilde{c}}_d\hat{\tilde{c}}_c. \tag{S10}$$

The grand potential can be written with the transformed operators as

$$\Omega^{\hat{W}}_{\beta,\mu}[\boldsymbol{U}^{\dagger}\tilde{\boldsymbol{h}}\boldsymbol{U}] = -\frac{1}{\beta}\ln\left({\rm Tr}e^{-\beta(\hat{W}-\mu\hat{N}+\sum_{a,b}\tilde{h}_{a,b}\hat{\tilde{c}}^{\dagger}_a\hat{\tilde{c}}_b)}\right) \tag{S11}$$

and thus

$$\Omega^{\hat{W}}_{\beta,\mu}[\boldsymbol{U}^{\dagger}\tilde{\boldsymbol{h}}\boldsymbol{U}] = \Omega^{\hat{W}}_{\beta,\mu}[\tilde{\boldsymbol{h}}] \tag{S12}$$

holds. Equation (S5) can thus be written as

$$F^{\hat{W}}_{\beta}[\boldsymbol{U}^{\dagger}\boldsymbol{\rho}\boldsymbol{U}] = \max_{\tilde{\boldsymbol{h}},\mu} \left[\Omega^{\hat{W}}_{\beta,\mu}[\tilde{\boldsymbol{h}}] - {\rm Tr}(\boldsymbol{\rho}\tilde{\boldsymbol{h}})\right] \tag{S13}$$

$$= F^{\hat{W}}_{\beta}[\boldsymbol{\rho}] \tag{S14}$$

concluding the proof.

## II. PRACTICAL CONSTRUCTION OF THE TRANSFORMATION

### A. One unitary transformation step

We iteratively construct the unitary transformation of the bath states discussed in section III A such that the one-particle reduced density matrix is a band matrix with a minimal bandwidth as given in Eq. (16). In this section we describe one iteration step. For that purpose, we write the one-particle reduced density matrix in block-form as in Eq. (12),

$$\boldsymbol{\rho} = \begin{pmatrix} \boldsymbol{\rho}_{\text{imp,imp}} & \boldsymbol{\rho}_{\text{imp,bath}} \\ \boldsymbol{\rho}^{\dagger}_{\text{imp,bath}} & \boldsymbol{\rho}_{\text{bath,bath}} \end{pmatrix} \tag{S15}$$

$$= \begin{pmatrix} \boldsymbol{\rho}_{\text{imp,imp}} & \boldsymbol{\rho}_{\text{imp,bath}_1} & \boldsymbol{\rho}_{\text{imp,rest}_1} \\ \boldsymbol{\rho}^{\dagger}_{\text{imp,bath}_1} & \boldsymbol{\rho}_{\text{bath}_1\text{,bath}_1} & \boldsymbol{\rho}_{\text{bath}_1\text{,rest}_1} \\ \boldsymbol{\rho}^{\dagger}_{\text{imp,rest}_1} & \boldsymbol{\rho}^{\dagger}_{\text{bath}_1\text{,rest}_1} & \boldsymbol{\rho}_{\text{rest}_1\text{,rest}_1} \end{pmatrix}, \tag{S16}$$

where the block imp consists of $N_{\text{imp}}$ interacting states making up the impurity. The block $\text{bath}_1$ contains $N_{\text{bath}_1}$ states and the block $\text{rest}_1$ the remaining $N_{\text{rest}_1}$ states. Transforming the one-particle basis with a block-diagonal unitary transformation defined in Eq. (15)

$$\boldsymbol{U} = \begin{pmatrix} \mathbf{1}_{N_{\text{imp}}} & \mathbf{0} \\ \mathbf{0} & \boldsymbol{U}_{\text{bath}} \end{pmatrix} \tag{S17}$$

$$= \begin{pmatrix} \mathbf{1}_{N_{\text{imp}}} & \mathbf{0} & \mathbf{0} \\ \mathbf{0} & \boldsymbol{U}_{\text{bath}_1\text{,bath}_1} & \boldsymbol{U}_{\text{bath}_1\text{,rest}_1} \\ \mathbf{0} & \boldsymbol{U}_{\text{rest}_1\text{,bath}_1} & \boldsymbol{U}_{\text{rest}_1\text{,rest}_1} \end{pmatrix} \tag{S18}$$

gives the transformed density matrix

$$\tilde{\boldsymbol{\rho}} = \boldsymbol{U}^{\dagger}\boldsymbol{\rho}\boldsymbol{U} = \begin{pmatrix} \boldsymbol{\rho}_{\text{imp,imp}} & \tilde{\boldsymbol{\rho}}_{\text{imp,bath}_1} & \tilde{\boldsymbol{\rho}}_{\text{imp,rest}_1} \\ \tilde{\boldsymbol{\rho}}^{\dagger}_{\text{imp,bath}_1} & \tilde{\boldsymbol{\rho}}_{\text{bath}_1\text{,bath}_1} & \tilde{\boldsymbol{\rho}}_{\text{bath}_1\text{,rest}_1} \\ \tilde{\boldsymbol{\rho}}^{\dagger}_{\text{imp,rest}_1} & \tilde{\boldsymbol{\rho}}^{\dagger}_{\text{bath}_1\text{,rest}_1} & \tilde{\boldsymbol{\rho}}_{\text{rest}_1\text{,rest}_1} \end{pmatrix}, \tag{S19}$$

with

$$\tilde{\boldsymbol{\rho}}_{\text{imp,rest}_1} = \boldsymbol{\rho}_{\text{imp,bath}_1}\boldsymbol{U}_{\text{bath}_1\text{,rest}_1} + \boldsymbol{\rho}_{\text{imp,rest}_1}\boldsymbol{U}_{\text{rest}_1\text{,rest}_1}. \tag{S20}$$

The unitary matrix $\boldsymbol{U}_{\text{bath}}$ is thus defined by

$$\boldsymbol{\rho}_{\text{imp,bath}_1}\boldsymbol{U}_{\text{bath}_1\text{,rest}_1} + \boldsymbol{\rho}_{\text{imp,rest}_1}\boldsymbol{U}_{\text{rest}_1\text{,rest}_1} = 0 \tag{S21}$$

This equation has the form of a bi-orthogonality condition. The matrices $\boldsymbol{\rho}_{\text{imp,bath}_1}$ and $\boldsymbol{\rho}_{\text{imp,rest}_1}$ define a set of $N_{\text{imp}}$ vectors $\boldsymbol{a}_i$ of dimension $N_{\text{imp}} + N_{\text{bath}_1}$. The matrices $\boldsymbol{U}_{\text{bath}_1\text{,rest}_1}$, $\boldsymbol{U}_{\text{bath}_1\text{,bath}_1}$ and $\boldsymbol{U}_{\text{rest}_1\text{,rest}_1}$ are then obtained from a second set of vectors $\boldsymbol{b}_i$, which are chosen orthonormal among each other and pairwise orthogonal to the first set, i.e.

$$\boldsymbol{a}_i\boldsymbol{b}_j = 0 \qquad \text{and} \qquad \boldsymbol{b}_i\boldsymbol{b}_j = \delta_{i,j}. \tag{S22}$$

We obtain the vectors $\boldsymbol{b}_j$ from a set of linearly independent vectors of dimension $N_{\text{bath}_1} + N_{\text{rest}_1}$ by first projecting out the vectors $\boldsymbol{a}_i$. In a second step, the resulting vectors are orthonormalized among each other using a Gram-Schmidt procedure.

The rank of the matrix $(\boldsymbol{\rho}_{\text{imp,bath}_1}\ \boldsymbol{\rho}_{\text{imp,rest}_1})$ has to be identical to the rank of $\tilde{\boldsymbol{\rho}}_{\text{imp,bath}_1}$. Thereby the lower bound of the number of states $N_{\text{bath}_1}$ in block $\text{bath}_1$ is given by the rank of $(\boldsymbol{\rho}_{\text{imp,bath}_1}\ \boldsymbol{\rho}_{\text{imp,rest}_1})$, which is equal to or smaller than the number of interacting states $N_{\text{imp}}$. For an efficient minimization over the one-particle reduced density matrix in Eq. (5) derivatives of the density-matrix functional with respect to the density matrix are essential. With the Gram-Schmidt-like orthogonalisation used in the transformation of the density matrix all derivatives are accessible in a computationally efficient way. As result we obtain a unitary transformation $\boldsymbol{U}$ of the one-particle basis, that brings any given one-particle reduced density matrix into the form

$$\tilde{\boldsymbol{\rho}} = \boldsymbol{U}^{\dagger}\boldsymbol{\rho}\boldsymbol{U} = \begin{pmatrix} \boldsymbol{\rho}_{\text{imp,imp}} & \tilde{\boldsymbol{\rho}}_{\text{imp,bath}_1} & \mathbf{0} \\ \tilde{\boldsymbol{\rho}}^{\dagger}_{\text{imp,bath}_1} & \tilde{\boldsymbol{\rho}}_{\text{bath}_1\text{,bath}_1} & \tilde{\boldsymbol{\rho}}_{\text{bath}_1\text{,rest}_1} \\ \mathbf{0} & \tilde{\boldsymbol{\rho}}^{\dagger}_{\text{bath}_1\text{,rest}_1} & \tilde{\boldsymbol{\rho}}_{\text{rest}_1\text{,rest}_1} \end{pmatrix}. \tag{S23}$$

The interacting one-particle states can only have non-zero one-particle density matrix elements with each other and with the $N_{\text{bath}_1} \leq N_{\text{imp}}$ non-interacting states of the first level effective bath.

### B. Iterated transformations

The construction scheme for the unitary transformation of the previous section can now be applied iteratively. For that purpose we only consider the states from block $\text{bath}_1$ and $\text{rest}_1$, i.e. the submatrix of the transformed density matrix in Eq. (S23)

$$\tilde{\boldsymbol{\rho}}_{\text{bath}_1\cup\text{rest}_1} = \begin{pmatrix} \tilde{\boldsymbol{\rho}}_{\text{bath}_1\text{,bath}_1} & \tilde{\boldsymbol{\rho}}_{\text{bath}_1\text{,rest}_1} \\ \tilde{\boldsymbol{\rho}}^{\dagger}_{\text{bath}_1\text{,rest}_1} & \tilde{\boldsymbol{\rho}}_{\text{rest}_1\text{,rest}_1} \end{pmatrix}. \tag{S24}$$

The block $\text{rest}_1$ is divided into a block $\text{bath}_2$ with

$$N_{\text{bath}_2} = rk(\tilde{\rho}_{\text{bath}_1\text{,rest}_1}) \leq N_{\text{bath}_1} \leq N_{\text{imp}} \tag{S25}$$

states as the second level effective bath and a block $\text{rest}_2$ with the remaining states. We arrive at the initial situation analogously to Eq. (S15), i.e.

$$\tilde{\boldsymbol{\rho}}_{\text{bath}_1\cup\text{rest}_1} = \begin{pmatrix} \tilde{\boldsymbol{\rho}}_{\text{bath}_1\text{,bath}_1} & \tilde{\boldsymbol{\rho}}'_{\text{bath}_1\text{,bath}_2} & \tilde{\boldsymbol{\rho}}'_{\text{bath}_1\text{,rest}_2} \\ (\tilde{\boldsymbol{\rho}}'_{\text{bath}_1\text{,bath}_2})^{\dagger} & \tilde{\boldsymbol{\rho}}'_{\text{bath}_2\text{,bath}_2} & \tilde{\boldsymbol{\rho}}'_{\text{bath}_2\text{,rest}_2} \\ (\tilde{\boldsymbol{\rho}}'_{\text{bath}_1\text{,rest}_2})^{\dagger} & (\tilde{\boldsymbol{\rho}}'_{\text{bath}_2\text{,rest}_2})^{\dagger} & \tilde{\boldsymbol{\rho}}'_{\text{rest}_2\text{,rest}_2} \end{pmatrix}. \tag{S26}$$

Now we can apply the scheme given in the previous section to construct the matrix

$$\boldsymbol{U}_2 = \begin{pmatrix} \mathbf{1}_{N_{\text{bath}_1}} & \mathbf{0} \\ \mathbf{0} & \boldsymbol{U}_{\text{bath}_2} \end{pmatrix} \tag{S27}$$

$$= \begin{pmatrix} \mathbf{1}_{N_{\text{bath}_1}} & \mathbf{0} & \mathbf{0} \\ \mathbf{0} & \boldsymbol{U}_{\text{bath}_2,\text{bath}_2} & \boldsymbol{U}_{\text{bath}_2,\text{rest}_2} \\ \mathbf{0} & \boldsymbol{U}_{\text{rest}_2,\text{bath}_2} & \boldsymbol{U}_{\text{rest}_2,\text{rest}_2} \end{pmatrix}, \tag{S28}$$

by solving the equation

$$\tilde{\boldsymbol{\rho}}'_{\text{bath}_1,\text{bath}_2}\boldsymbol{U}_{\text{bath}_2,\text{rest}_2} + \tilde{\boldsymbol{\rho}}'_{\text{bath}_1,\text{rest}_2}\boldsymbol{U}_{\text{rest}_2,\text{rest}_2} = \mathbf{0}. \tag{S29}$$

The construction yields the unitary matrix that transforms $\tilde{\boldsymbol{\rho}}_{\text{bath}_1\cup\text{rest}_1}$ to

$$\boldsymbol{U}_2^\dagger \tilde{\boldsymbol{\rho}}_{\text{bath}_1\cup\text{rest}_1}\boldsymbol{U}_2 = \tag{S30}$$

$$\begin{pmatrix} \tilde{\boldsymbol{\rho}}_{\text{bath}_1,\text{bath}_1} & \tilde{\boldsymbol{\rho}}_{\text{bath}_1,\text{bath}_2} & \mathbf{0} \\ \tilde{\boldsymbol{\rho}}^\dagger_{\text{bath}_1,\text{bath}_2} & \tilde{\boldsymbol{\rho}}_{\text{bath}_2,\text{bath}_2} & \tilde{\boldsymbol{\rho}}_{\text{bath}_2,\text{rest}_2} \\ 0 & \tilde{\boldsymbol{\rho}}^\dagger_{\text{bath}_2,\text{rest}_2} & \tilde{\boldsymbol{\rho}}_{\text{rest}_2,\text{rest}_2} \end{pmatrix}. \tag{S31}$$

Combining the two unitary transformations $\boldsymbol{U}$ from Eq. (S23) and $\boldsymbol{U}_2$ from Eq. (S27) yields

$$\tilde{\boldsymbol{\rho}} = \begin{pmatrix} \mathbf{1}_{N_{\text{imp}}} & \mathbf{0} \\ \mathbf{0} & \boldsymbol{U}_2^\dagger \end{pmatrix} \boldsymbol{U}^\dagger \boldsymbol{\rho} \boldsymbol{U} \begin{pmatrix} \mathbf{1}_{N_{\text{imp}}} & \mathbf{0} \\ \mathbf{0} & \boldsymbol{U}_2 \end{pmatrix} \tag{S32}$$

$$= \begin{pmatrix} \boldsymbol{\rho}_{\text{imp,imp}} & \tilde{\boldsymbol{\rho}}_{\text{imp,bath}_1} & \mathbf{0} & \mathbf{0} \\ \tilde{\boldsymbol{\rho}}^\dagger_{\text{imp,bath}_1} & \tilde{\boldsymbol{\rho}}_{\text{bath}_1,\text{bath}_1} & \tilde{\boldsymbol{\rho}}_{\text{bath}_1,\text{bath}_2} & \mathbf{0} \\ \mathbf{0} & \tilde{\boldsymbol{\rho}}^\dagger_{\text{bath}_1,\text{bath}_2} & \tilde{\boldsymbol{\rho}}_{\text{bath}_2,\text{bath}_2} & \tilde{\boldsymbol{\rho}}_{\text{bath}_2,\text{rest}_2} \\ \mathbf{0} & \mathbf{0} & \tilde{\boldsymbol{\rho}}^\dagger_{\text{bath}_2,\text{rest}_2} & \tilde{\boldsymbol{\rho}}_{\text{rest}_2,\text{rest}_2} \end{pmatrix}.$$

Iterating this scheme leads to the band matrix given in Eq. (16), where the upper bound for the bandwidth is given by the number of interacting states $N_{\text{imp}}$. The $n$-th level effective bath $\text{bath}_n$ consists of $N_{\text{bath}_n}$ states and the relation $N_{\text{imp}} \geq N_{\text{bath}_1} \geq N_{\text{bath}_2} \geq ...$ holds. Thus proving the relation given in sec. III A.

## III. EXACT DECOUPLING

Here we prove a relation between the eigenvalue spectrum of the bath-density matrix and the discarded weight discussed in sec. III C: If the eigenvalue spectrum of the bath-density matrix consists of $N$ distinct values with a $n_j$-fold degeneracy each, then there is a number of effective bath states $N_{\text{bath}} \leq \sum_{j=1}^{N} \min(n_j, N_{\text{imp}})$ for which the discarded weight $\sigma_{N_{\text{imp}}+N_{\text{bath}}}(\tilde{\boldsymbol{\rho}})$ of the transformed density matrix $\tilde{\boldsymbol{\rho}}$ vanishes. To prove this relation, we write the one-particle reduced density matrix $\boldsymbol{\rho}$ in a block-form as in Eq. (12)

$$\boldsymbol{\rho} = \begin{pmatrix} \boldsymbol{\rho}_{\text{imp,imp}} & \boldsymbol{\rho}_{\text{imp,bath}} \\ \boldsymbol{\rho}^\dagger_{\text{imp,bath}} & \boldsymbol{\rho}_{\text{bath,bath}} \end{pmatrix}, \tag{S33}$$

where $\boldsymbol{\rho}_{\text{imp,imp}} \in \mathbb{C}^{N_{\text{imp}}\times N_{\text{imp}}}$ and $\boldsymbol{\rho}_{\text{bath,bath}} \in \mathbb{C}^{N_{\text{bath}}\times N_{\text{bath}}}$. By diagonalization of the bath-density matrix $\boldsymbol{\rho}_{\text{bath,bath}}$ any density matrix can transformed to the shape

$$\tilde{\boldsymbol{\rho}} = \boldsymbol{U}^\dagger \boldsymbol{\rho} \boldsymbol{U} = \begin{pmatrix} \boldsymbol{\rho}_{\text{imp,imp}} & \tilde{\boldsymbol{\rho}}_{\lambda,\text{imp,bath}} \\ \tilde{\boldsymbol{\rho}}^\dagger_{\lambda,\text{imp,bath}} & \text{diag}(\lambda_1, ..., \lambda_{N_{\text{bath}}}) \end{pmatrix}. \tag{S34}$$

Here $\text{diag}(\lambda_1, ..., \lambda_{N_{\text{bath}}})$ stands for the real matrix with the ordered eigenvalues $\lambda_1, ..., \lambda_{N_{\text{bath}}}$ of $\boldsymbol{\rho}_{\text{bath,bath}}$ on the diagonal. No additional properties of $\tilde{\boldsymbol{\rho}}_{\lambda,\text{imp,bath}}$ are assumed. Thus the following discussion is valid for any hermitian matrix $\boldsymbol{\rho}$.

Now we assume that the eigenvalue spectrum of the bath density matrix $\boldsymbol{\rho}_{\text{bath,bath}}$ consists of $N$ distinct values $\Lambda_1, ..., \Lambda_N$ with the degeneracies $n_1, \; ... \;, n_N$, i.e. $\Lambda_1 = \lambda_1 = ... = \lambda_{n_1}$. If we consider a single set of degenerate eigenvalues with the index $j \in \{1, ..., N\}$ we can write the rows and columns corresponding to this set as

$$\tilde{\boldsymbol{\rho}} = \left(\begin{array}{cc|c|c} \boldsymbol{\rho}_{\text{imp,imp}} & \cdots & \tilde{\boldsymbol{\rho}}_{\lambda,\text{imp,bath}_j} & \cdots \\ \vdots & \cdots & \mathbf{0} & \cdots \\ \hline \tilde{\boldsymbol{\rho}}^\dagger_{\lambda,\text{imp,bath}_j} & \mathbf{0} & \Lambda_j \mathbf{1}_{n_j\times n_j} & \mathbf{0} \\ \hline \vdots & \cdots & \mathbf{0} & \cdots \end{array}\right), \tag{S35}$$

with $\tilde{\boldsymbol{\rho}}_{\lambda,\text{imp,bath}}$ in Eq. (S34) written as $\tilde{\boldsymbol{\rho}}_{\lambda,\text{imp,bath}} = (\tilde{\boldsymbol{\rho}}_{\lambda,\text{imp,bath}_1} \; \cdots \; \tilde{\boldsymbol{\rho}}_{\lambda,\text{imp,bath}_N})$. Within each $n_j$-dimensional eigenspace for the eigenvalue $\Lambda_j$ we can perform a unitary transformation $\boldsymbol{U}'_j$, i.e. in total the block-diagonal unitary transformation $\boldsymbol{U}'$

$$\boldsymbol{U}' = \begin{pmatrix} \mathbf{1}_{N_{\text{imp}}} & \mathbf{0} & \cdots & \\ \mathbf{0} & \boldsymbol{U}'_1 & \mathbf{0} & \cdots \\ \vdots & & \ddots & \\ \mathbf{0} & \cdots & \mathbf{0} & \boldsymbol{U}'_N \end{pmatrix}. \tag{S36}$$

The unitary matrices $\boldsymbol{U}'_j$ of the separate blocks are now chosen, so that they transform $\tilde{\boldsymbol{\rho}}_{\lambda,\text{imp,bath}_j}$ in Eq. (S35) as

$$\begin{pmatrix} \tilde{\boldsymbol{\rho}}'_{\lambda,\text{imp,bath},j} & \mathbf{0} \end{pmatrix} = \tilde{\boldsymbol{\rho}}_{\lambda,\text{imp,bath}_j}\boldsymbol{U}_j, \tag{S37}$$

where $\tilde{\boldsymbol{\rho}}'_{\lambda,\text{imp,bath},j}$ should have the least possible number of columns, that we denote with with $n'_j$. The upper bound for the number of columns of the matrix $\tilde{\boldsymbol{\rho}}'_{\lambda,\text{imp,bath}_j}$ can be deduced as follows:

- If $n_j \leq N_{\text{imp}}$, then $n'_j = rk(\tilde{\boldsymbol{\rho}}_{\lambda,\text{imp,bath}_j}) \leq n_j$ holds.
- In case $n_j > N_{\text{imp}}$, we have $n'_j = rk(\tilde{\boldsymbol{\rho}}_{\lambda,\text{imp,bath}_j}) \leq N_{\text{imp}}$.

We then obtain the form

$$\tilde{\boldsymbol{\rho}}' = (\boldsymbol{U}')^\dagger \tilde{\boldsymbol{\rho}} \boldsymbol{U}' = \left(\begin{array}{cc|cc|c} \boldsymbol{\rho}_{\mathrm{imp,imp}} & \dots & \tilde{\boldsymbol{\rho}}'_{\lambda,\mathrm{imp,bath},j} & \mathbf{0} & \dots \\ \vdots & \dots & \mathbf{0} & \mathbf{0} & \dots \\ \hline (\tilde{\boldsymbol{\rho}}'_{\lambda,\mathrm{imp,bath},j})^\dagger & \mathbf{0} & \Lambda_j \mathbf{1}_{n'_j \times n'_j} & \mathbf{0} & \mathbf{0} \\ \mathbf{0} & \mathbf{0} & \mathbf{0} & \Lambda_j \mathbf{1}_{n_j - n'_j \times n_j - n'_j} & \mathbf{0} \\ \hline \vdots & \dots & \mathbf{0} & \mathbf{0} & \dots \end{array}\right). \tag{S38}$$

Basis states corresponding to blocks with $\Lambda_j \mathbf{1}_{n_j - n'_j \times n_j - n'_j}$ do not couple to other basis states and can be neglected. So that the upper bound for number of the remaining bath basis states is given by

$$\sum_{j=1}^{N} n'_j = \sum_{j=1}^{N} \min\left[n_j, rk(\tilde{\boldsymbol{\rho}}_{\lambda,\mathrm{imp,bath}_j})\right]. \tag{S39}$$

We have shown that an arbitrary density matrix with an impurity of $N_{\mathrm{imp}}$ states and $N$ disjoint sets of $n_j$-fold degenerate eigenvalues of the bath-density matrix can be exactly decoupled if the number of effective bath basis states is at least $\sum_{j=1}^{N} \min\left[n_j, rk(\tilde{\boldsymbol{\rho}}_{\lambda,\mathrm{imp,bath}_j})\right]$. The upper bound is given by $\sum_{j=1}^{N} \min(n_j, N_{\mathrm{imp}})$, when all $\tilde{\boldsymbol{\rho}}_{\lambda,\mathrm{imp,bath}_j}$ have full column rank. In the case of $N_{\mathrm{imp}} = 2$, that is a two-spin-orbital impurity, and a non-spin-polarized density matrix, i.e. $n_j \geq 2$, we obtain an upper bound for the number of effective bath sites equal to the number $N$ of disjoint sets of degenerate eigenvalues of the bath density matrix. Because of the construction of the unitary transformations via a Gram-Schmidt-like orthogonalisation scheme, the ACA does not rely on a degeneracy of the eigenvalues of the bath-density matrix, which would be problematic in a numerical treatment. If the eigenvalues of the bath-density matrix are not degenerate within groups, but form $N$ clusters with small but finite spreads, the ACA transformation results in a finite, but very small discarded weight after $N$ effective bath levels.

## IV. EVALUATION OF THE EXACT DENSITY-MATRIX FUNCTIONAL

We evaluate the density-matrix functional $F^{\hat{W}}[\boldsymbol{\rho}]$ via Levy's constrained-search algorithm:

$$F^{\hat{W}}[\boldsymbol{\rho}] = \min_{\{P_i, |\Psi_i\rangle\} \to \boldsymbol{\rho}} \sum_i P_i \langle \Psi_i | \hat{W} | \Psi_i \rangle. \tag{S40}$$

This describes a constrained minimization over an ensemble of $N_\Psi$ many-particle wave functions $|\Psi_i\rangle$ and ensemble probabilities $P_i$. The many-particle wave functions $|\Psi_i\rangle$ have to be orthonormal, the ensemble probabilities have to be positive and sum up to one. Furthermore, the ensemble of many-particle wave functions and the probabilities have to generate the given one-particle density matrix $\boldsymbol{\rho} \in \mathbb{C}^{N_\chi \times N_\chi}$ according to

$$\rho_{b,a} = \sum_i P_i \langle \Psi_i | \hat{c}_a^\dagger \hat{c}_b | \Psi_i \rangle. \tag{S41}$$

At this point we have to choose some parametrization of the many-particle wave functions. For the calculations presented in this paper we used a full configuration interaction representations in occupation number representation, i.e.

$$|\Psi_i\rangle = \sum_j a_{i,j} |n_{1,j} n_{2,j} \dots n_{N_\chi,j}\rangle \tag{S42}$$

$$= a_{i,1}|000\dots\rangle + a_{i,2}|100\dots\rangle + a_{i,3}|010\dots\rangle + . \tag{S43}$$

Here $n_{\alpha,j} \in \{0,1\}$ is the occupation of the $\alpha$-th one-particle basis state in the $j$-th many-particle basis state. There are $2^{N_\chi}$ basis states in the many-particle basis. Thus, a many-particle wave function $|\Psi_i\rangle$ is parametrized via $2^{N_\chi}$ complex coefficients $a_{i,j}$. The inequality constraints on the ensemble probabilities $P_i$, that is $0 \leq P_i$, are translated into auxiliary unconstrained variables $p_i$ with $P_i = p_i^2$. We define a vector of variational parameters $\vec{x}$, which contains the $N_\Psi 2^{N_\chi}$ complex variables $a_i$ and the $N_\Psi$ auxiliary real parameters $p_i$. $N_\Psi$ denotes the number of many-particle wave functions in the ensemble.

In the spirit of mathematical programming, we write down the objective function $f(\vec{x})$ and equality constraints $c_j(\vec{x}) = 0$ separately:

$$f(\vec{x}) = \sum_i P_i(\vec{x}) \langle \Psi_i(\vec{x}) | \hat{W} | \Psi_i(\vec{x}) \rangle \tag{S44}$$

$$c_0(\vec{x}) = \sum_i P_i(\vec{x}) - 1 \tag{S45}$$

$$c_{ij}(\vec{x}) = \langle \Psi_i(\vec{x}) | \Psi_j(\vec{x}) \rangle - \delta_{ij} \tag{S46}$$

$$c_{ab}(\vec{x}) = \sum_i P_i \langle \Psi_i(\vec{x}) | \hat{c}_a^\dagger \hat{c}_b | \Psi_i(\vec{x}) \rangle - \rho_{b,a} \tag{S47}$$

In total there are $N_\Psi^2 + N_\chi^2 + 1$ real equality constrains and $2N_\Psi 2^{N_\chi} + N_\Psi$ real variational parameters. We have found the primal Powell-Hestenes Augmented Lagrangian[1–3] to work efficiently and reliably for the resulting constrained optimization. The augmented Lagrangian combines a quadratic penalty method with the Lagrangian of the problem. For a general equality constrained minimization problem (objective $f$, constraints $c_i(\vec{x}) = 0$) we set up the augmented Lagrangian

$L_A(\vec{x}, \vec{\lambda}, \vec{\mu})$

$$L_A(\vec{x}, \vec{\lambda}, \vec{\mu}) = f(\vec{x}) - \sum_i \lambda_i c_i(\vec{x}) + \frac{1}{2}\sum_i \mu_i c_i^2(\vec{x}), \quad \text{(S48)}$$

where $\lambda_i$ are the Lagrange parameters and $\mu_i$ are the penalty parameters.

First some parameters must be chosen, like the minimal desired minimization tolerance $\tau_{min}$, the minimal desired constrained violation $\sigma_{min}$, as well as multiplication factors for minimization tolerance $\tau_f < 1$, constraint violation tolerance $\sigma_f < 1$ and penalty $\mu_f > 1$. The algorithm is rather robust when it comes to choices for theses parameters. However tuning these parameters can strongly influence the runtime. Care has to be taken that the penalty parameters do not increase too quickly, because that can lead to problems with floating point precision so that the unconstrained minimization can become ill-conditioned and take a long time to converge. However, the main problem of quadratic penalty methods, namely the need to raise the penalty parameter to infinity, does not exists for the augmented Lagrangian method. It can be shown[3] that, when some mild additional requirements are fulfilled, there is a finite threshold penalty parameter $\overline{\mu}$ such that for all penalties $\mu_i \geq \overline{\mu}$ the minimizer of the constrained problem $\vec{x}^*$ is also a minimizer of the unconstrained problem $\min_{\vec{x}} L_a(\vec{x}, \vec{\lambda}^*, \vec{\mu})$ with the exact Lagrange multipliers $\vec{\lambda}^*$.

Starting from an initial choice of the variational parameters $\vec{x}_{(0)}$, $\vec{\lambda}_1$, $\vec{\mu}_1$, the minimization tolerance $\tau_1 > 0$ and constraint violation tolerance $\sigma_1 > 0$, the algorithm works as follows

- For every outer iteration k=1,2,.... do:
  - perform an unconstrained minimization of

    $$\min_{\vec{x}} L_A(\vec{x}, \vec{\lambda}_k, \vec{\mu}_k) \quad \text{(S49)}$$

    from the starting point $\vec{x}_{k-1}$ with convergence tolerance $\tau_k$ for $|\nabla_{\vec{x}} L_A(\vec{x}, \vec{\lambda}_k, \vec{\mu}_k)|$ and use the resulting minimizer $\vec{x}^*$ as $\vec{x}_k$,
  - update Lagrange multipliers with first order multiplier update

    $$\lambda_{k+1,i} = \lambda_{k,i} - \mu_{k,i} c_i(\vec{x}_k), \quad \text{(S50)}$$

  - if $\max |c_i(\vec{x}_k)| \leq \sigma_k$, then
    * set $\tau_{k+1} = \max(\tau_f \tau_k, \tau_{min})$
    * set $\sigma_{k+1} = \max(\sigma_f \sigma_k, \sigma_{min})$
    * do for all i: if $|c_i(\vec{x}_k)| \leq \sigma_{k+1}$ then set $\mu_{k+1,i} = \mu_{k,i}/\mu_f^{0.1}$
  - if $\max |c_i(\vec{x}_k)| > \sigma_k$, then
    * do for all i: if $|c_i(\vec{x}_k)| \leq \sigma_{k+1}$ then set $\mu_{k+1,i} = \mu_{k,i}/\mu_f^{0.1}$ or else set $\mu_{k+1,i} = \mu_{k,i} \cdot \mu_f$
- check if the constraint violations $c_i(\vec{x}_k)$ are sufficiently small and is $|\nabla_{\vec{x}} L_A(\vec{x}, \vec{\lambda}_k, \vec{\mu}_k)|$ is smaller then the convergence threshold. If this is true, then stop. Then $\vec{x}_k$ is the solution for the variational parameters and $\vec{\lambda}_k$ for the Lagrange multipliers.

The derivatives of the density-matrix functional with respect to the density matrix are given by the resulting Lagrange multipliers. We use the complex-generalized variant[4] of the limited-memory Broyden-Fletcher-Goldfarb-Shanno (L-BFGS[5–8]) for the unconstrained minimization step. Usually with a memory parameter of $m = 10$. This algorithm usually converges after about 10-30 outer iterations. It can be warm-started with the minimum from the previous density-matrix functional-calculation and does not suffer from the Maratos effect. A discussion of the Maratos effect can be found in[3]. The fact that it does only use matrix-vector operations and no matrix factorization makes it very suitable for very large scale constrained optimization. Our implementation is based on sparse matrix-vector algebra and has been used with many-particle wave functions with up to $5 \cdot 10^7$ Slater determinants on a desktop computer for the case of a single many-particle wave function $N_\Psi = 1$.

In the present study we used a convergence threshold of $10^{-4}t$ for all calculations except for the case of the bandwidth dependence of the single-impurity Anderson model, where we have used $10^{-4}V$. The threshold for the constraint violations $c_i(\vec{x}_k)$ was chosen as $10^{-6}$. The results shown in this paper have been obtained with the density-matrix functional with only one many-particle wave function $F^{\hat{W}}_{\text{single } |\Psi\rangle}$ of Eq. (7). It is not a priori clear if the density-matrix functional evaluated with one many-particle wave function $F^{\hat{W}}_{\text{single } |\Psi\rangle}$ of Eq. (7) is also identical to the ensemble density-matrix function $F^{\hat{W}}$ of Eq. (6) if used for a one-particle density matrix with truncated bath states and a system with an non-degenerate ground state. Our comparisons of numerical calculations have shown that even if there is a difference for the single-impurity Anderson model investigated here, it is smaller than the convergence criterion used. Thus the use of the simpler density-matrix functional $F^{\hat{W}}_{\text{single } |\Psi\rangle}$ while considerably reducing the computational effort does not introduce additional errors.

## V. SIAM IN ADDITIONAL PARAMETER REGIMES

### A. Impurity on-site-energy dependence

#### 1. *Exact results*

The dependence of the exact ground state and the ground state in the Hartree-Fock approximation on the impurity on-site energy $\epsilon_f$ for the single-impurity An-

derson model defined by Eq. (38)-(41) and $L_{\text{bath}} = 11$, $U/t = 8$, $t > 0$, $V/t = 0.4$ is shown in Fig. S1.

The behaviour of this model for different impurity on-site energies $\epsilon_f$ can be separated in three regions, depending on the relation of the on-site energy to the Fermi energy of the bath $\epsilon_{F,\text{bath}} \approx 0.28t$.

- For $\epsilon_f + U \ll \epsilon_{F,\text{bath}}$, the impurity is doubly occupied $n_f \approx 2$. The interaction energy takes the maximal possible value $W_{max} = U$.
- The range $\epsilon_f < \epsilon_{F,\text{bath}}$ and $\epsilon_{F,\text{bath}} < \epsilon_f + U$ is the Kondo regime. The impurity is approximately half filled, i.e. $n_f \approx 1$. The charge fluctuation on the impurity $\langle n_f^2 \rangle - \langle n_f \rangle^2$, is small in this region, so that the ground-state wave function has only a negligible contribution from states that are empty or doubly occupied on the impurity. In this region, the impurity can be described by an effective local spin-1/2-moment, that is coupled to the bath. This situation is identical to the Kondo model[9].
- For $\epsilon_f > \epsilon_{F,\text{bath}}$, the impurity is nearly empty.

The three energy regions are separated by mixed-valence regions. Here the impurity occupation switches rapidly from one integral occupation to another and the charge fluctuations on the impurity are thus large.

The unrestricted Hartree-Fock approximation is exact in the limits of a doubly occupied impurity $\epsilon_f \to -\infty$ and an empty impurity $\epsilon_f \to \infty$. In the intermediate region shown in Fig. S1 it qualitatively reproduces the three distinct regions, but suffers from an unphysical spin-symmetry breaking with a finite magnetic moment on the impurity $m_f > 0$ in the Kondo-regime.

Fig. S2 shows the eigenvalue spectrum of the bath density matrix of the exact ground state as function of the impurity on-site energy. Similarly to the interaction-strength dependence discussed in section V B we find here at most three distinct clusters of eigenvalues with very small spread, so that we expect the ACA with three effective bath sites, i.e. $M = 3$, to converge to the exact ground state within the convergence tolerance of the numerical minimization.

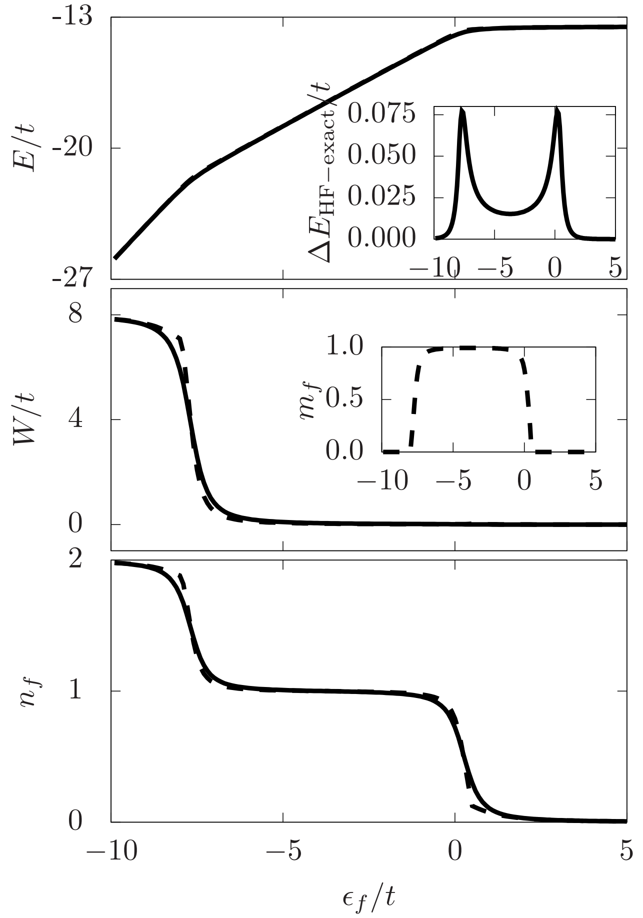


Supplementary Figure S1. Ground-state energy $E$, interaction energy $W$ and impurity occupation $n_f$ of the exact ground state (solid lines) and the unrestricted Hartree-Fock ground state (dashed lines) of the Hamiltonian defined Eq. (38)-(41) with $L_{\text{bath}} = 11$, $U/t = 8$, $t > 0$, $V/t = 0.4$ at half filling. The inset in the first graph shows the difference $\Delta E_{\text{HF}-\text{exact}} = E_{HF} - E_{\text{exact}}$ between the ground-state energy in the Hartree-Fock approximation and the exact result. The inset in the second graph shows the magnetic moment $m_f = n_{f,\uparrow} - n_{f,\downarrow}$ of the impurity within the Hartree-Fock approximation.

### *2. ACA results*

Let us compare the ACA with the exact result and the Hartree-Fock approximation. The ACA with truncation level $M = 3$ is again exact within the numerical precision of the solver for the density-matrix functional, and will not be discussed further in this section. Rather, we concentrate on the performance of the low truncation levels $M = 1$ and $M = 2$. The deviations of the ACA from the exact results are shown in Fig. S3. The ACA with low truncation levels $M = 1$ and $M = 2$ and the Hartree-Fock approximation describe the system well in the energy regions with the empty and the doubly occupied impurity. In the Kondo regime, the Hartree-Fock approximation describes the interaction energy well, but the predicted state is a broken symmetry state with a magnetized impurity. The ACA describes the physical state of Kondo regime correctly.

The good description of the Kondo regime indicates that the ACA copes well with static correlation, that is, with states that cannot be represented well with a single Slater determinant. The ACA inherits this feature from the constrained search, which constructs the density-matrix functional from a multi-configuration wave function. The largest deviations occur in the mixed-valence regimes at $\epsilon_f = \epsilon_{F,\text{bath}} - U \approx -7.7t$ and $\epsilon_f = \epsilon_{F,\text{bath}} \approx 0.28t$. Even for low truncation levels such as $M = 1$ and $M = 2$, the impurity occupation and the total energy deviate only by about 3 % from the exact value. The

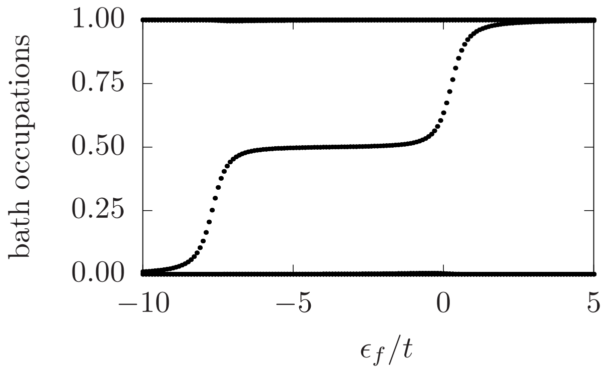


Supplementary Figure S2. Eigenvalue spectrum (occupations) of the bath density matrix $\boldsymbol{\rho}_{BB}$ of the exact ground state for the same model as in Fig. S1.

deviations in the total energy are one order of magnitude smaller than those of the interaction energy itself. The Müller correction (section III E) of the ACA improves the uncorrected ACA considerably, in particular in the mixed-valence regime where the deviations are largest.

### B. Bandwidth dependence

#### 1. *Exact results*

As discussed in section III C the ACA is exact for a SIAM in the limit of a vanishing bath bandwidth $t \to 0$ and in the limit of widely separated discrete bath levels $t \to \infty$. By varying the hopping $t$ in the bath, which is proportional to the bath bandwidth, we investigate these two limits. The dependence of the exact ground state and the ground state in the Hartree-Fock approximation on the bath hopping parameter $t$ for the single-impurity Anderson model defined by Eq. (38)-(41) and $L_{\text{bath}} = 11$, $U/V = 5$, $V > 0$, $\epsilon_f/V = -1$ is shown in Fig. S4. The exact total energy is approximately linear with the bath hopping parameter, because it is dominated by the one-particle energy of the bath. In the limit of degenerate bath levels, $t \to 0$, the Fermi energy of the bath vanishes $\epsilon_{F,\text{bath}} = 0$. In this limit the system is close to the transition from the singly occupied to the empty impurity, because of $\epsilon_f + U \gg \epsilon_{F,\text{bath}}$ and $\epsilon_f < \epsilon_{F,\text{bath}}$.

Increasing the bath hopping $t$ increases the distance of the bath-Fermi energy $\epsilon_{F,\text{bath}} \approx 0.28t$ to the impurity on-site energy $\epsilon_f = -V$, so that impurity occupation increases (see also Fig. S4). In the limit of widely separated discrete bath levels, $t \to \infty$, the impurity is doubly occupied and the interaction energy maximal, $W_{\text{exact}} = U$. Also in this parameter range the unrestricted Hartree-Fock approximation suffers from an unphysical spin-symmetry breaking. It becomes exact in the limit of widely separated discrete bath levels. The spectrum of the bath density matrix of the exact ground state in Fig. (S5), also shows three distinct clusters of

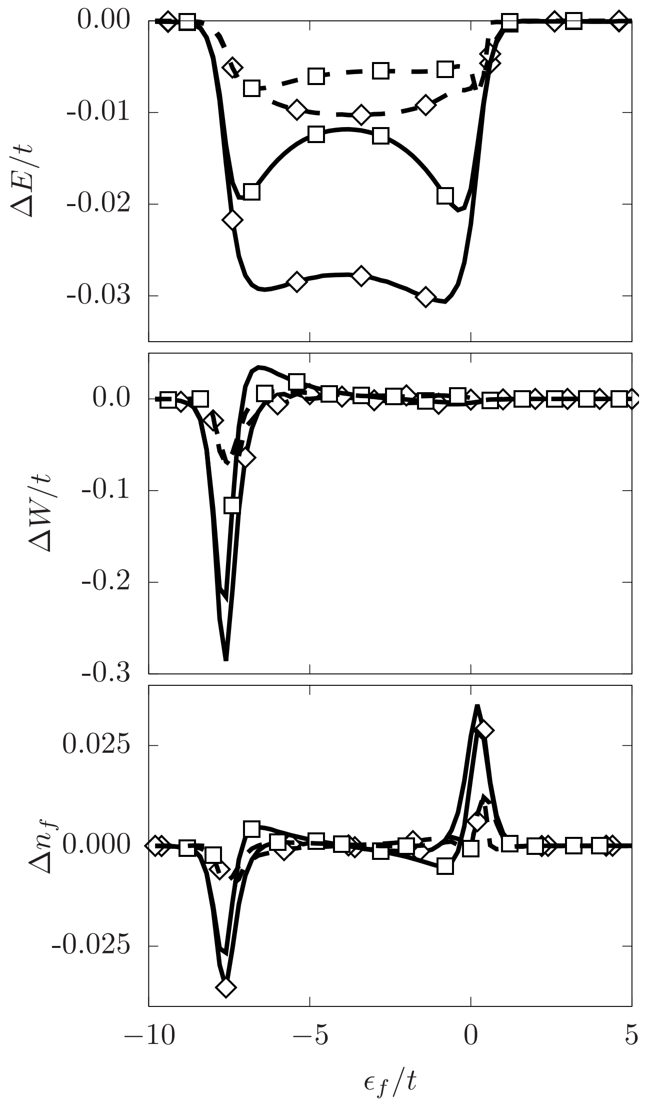


Supplementary Figure S3. Deviation of the ground-state energy $\Delta E = E_{(c)ACA(M)} - E_{\text{exact}}$, interaction energy $\Delta W = W_{(c)ACA(M)} - W_{\text{exact}}$ and impurity occupation $\Delta n_f = n_{f,(c)ACA(M)} - n_{f,\text{exact}}$ between the ground state within the (corrected) adaptive cluster approximation and the exact ground state. Same model as in Fig. S1.The corresponding exact results are shown in Fig. S1. Solid lines correspond to the uncorrected ACA and dashed lines to the Müller-corrected ACA results. Truncation with $M = 1$ (solid line with diamonds) and $M = 2$ (solid line with squares). The results for $M = 3$ are not shown, because they agree with the exact results within the convergence criteria.

eigenvalues for finite bath hopping parameters. Consequently the ACA with $M = 3$ will reproduce the exact ground state within the convergence tolerance of the numerical minimization. In the limit of vanishing bath bandwidth $t \to 0$ the cluster with fractional occupations has a large finite spread, so that the argument based on clusters of degenerate eigenvalues will not hold anymore.

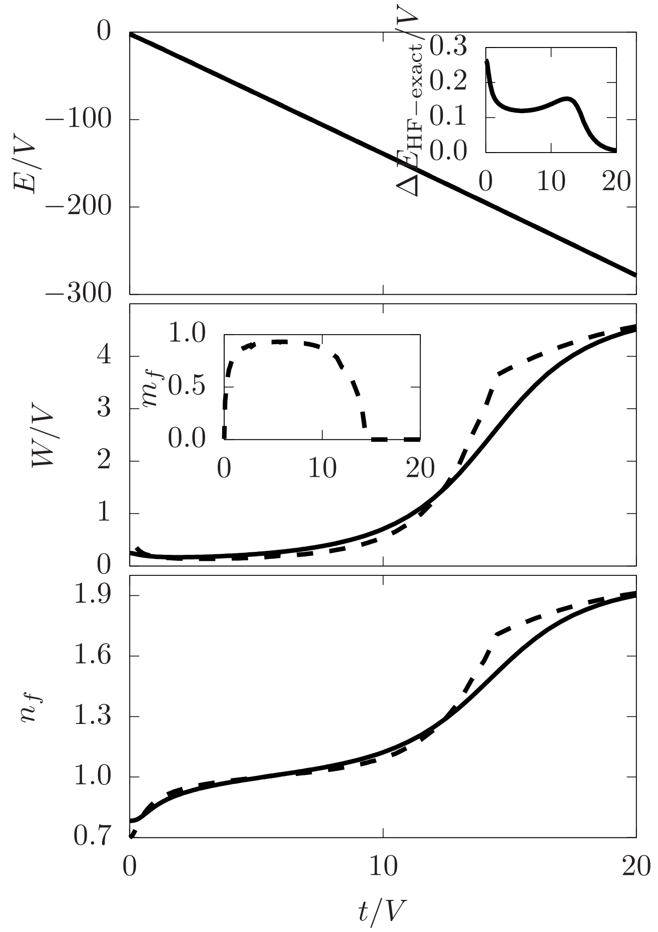


Supplementary Figure S4. Ground-state energy $E$, interaction energy $W$ and impurity occupation $n_f$ of the exact ground state (solid lines) and the unrestricted Hartree-Fock ground state (dashed lines) of the Hamiltonian defined Eq. (38)-(41) with $L_{\text{bath}} = 11$, $U/V = 5$, $V > 0$, $\epsilon_f/V = -1$ at half filling. The inset in the first graph shows the difference $\Delta E_{\text{HF}-\text{exact}} = E_{HF} - E_{\text{exact}}$ between the ground-state energy in the Hartree-Fock approximation and the exact result. The inset in the second graph shows the magnetic moment $m_f = n_{f,\uparrow} - n_{f,\downarrow}$ of the impurity within the Hartree-Fock approximation.

However the limit of vanishing bath bandwidth is already exactly described by the ACA with just one effective bath site, i.e. $M = 1$. This is due to the equivalence with the two-level approximation, which has been shown to be exact in this case[10].

### 2. ACA results

Figure S6 shows the deviations of the ground-state energy, interaction energy and impurity occupation within the (corrected) ACA with one and two effective bath sites from the exact results. The numerical results confirm that the uncorrected ACA with one effective bath site ($M = 1$) becomes exact in the limit of a vanishing bath

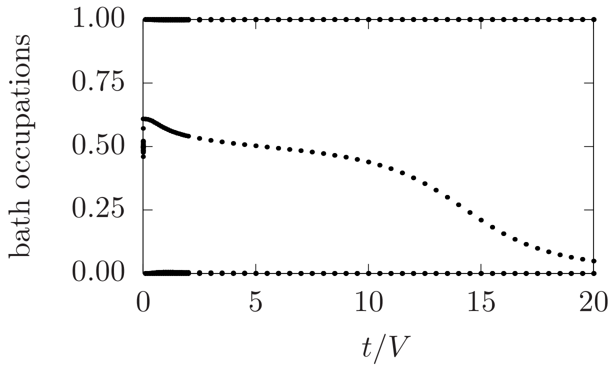


Supplementary Figure S5. Eigenvalue spectrum (occupations) of the bath density matrix $\boldsymbol{\rho}_{BB}$ of the exact ground state for the same model an in Fig. S4.

bandwidth $t \to 0$ and in the limit of widely separated bath levels $t \to \infty$ as discussed in section III C. Even though the interaction energy varies between very small values and $W \approx U$ in this parameter regime, we get small deviations of the interaction energy within the ACA over the whole range. Unfortunately the deviations are largest in the regime, where the impurity is approximately single occupied and the absolute value of the interaction energy is small. Also in this parameter regime we find a strong correlation between large deviations of the impurity occupation and large deviations in the total ground-state energy and interaction energy. The correction with the Müller functional reduces the deviation of the total energy by approximately a factor of two compared to the corresponding uncorrected ACA results.

* robert.schade@tu-clausthal.de

[1] M. Powell, Academic Press, NY , 283 (1969).
[2] M. R. Hestenes, J. Optim. Theory Appl. **4**, 303 (1969).
[3] J. Nocedal and S. Wright, *Numerical Optimization*, Springer Series in Operations Research and Financial Engineering (Springer New York, 2006).
[4] L. Sorber, M. V. Barel, and L. D. Lathauwer, SIAM Journal on Optimization **22**, 879 (2012), https://doi.org/10.1137/110832124.
[5] C. G. BROYDEN, IMA Journal of Applied Mathematics **6**, 76 (1970).
[6] R. Fletcher, The Computer Journal **13**, 317 (1970).
[7] D. Goldfarb, Math. Comp. **24**, 23 (1970).
[8] D. F. Shanno, Math. Comp. **24**, 647 (1970).
[9] J. Kondo, Progress of Theoretical Physics **32**, 37 (1964).
[10] W. Töws and G. M. Pastor, Phys. Rev. B **83**, 235101 (2011).

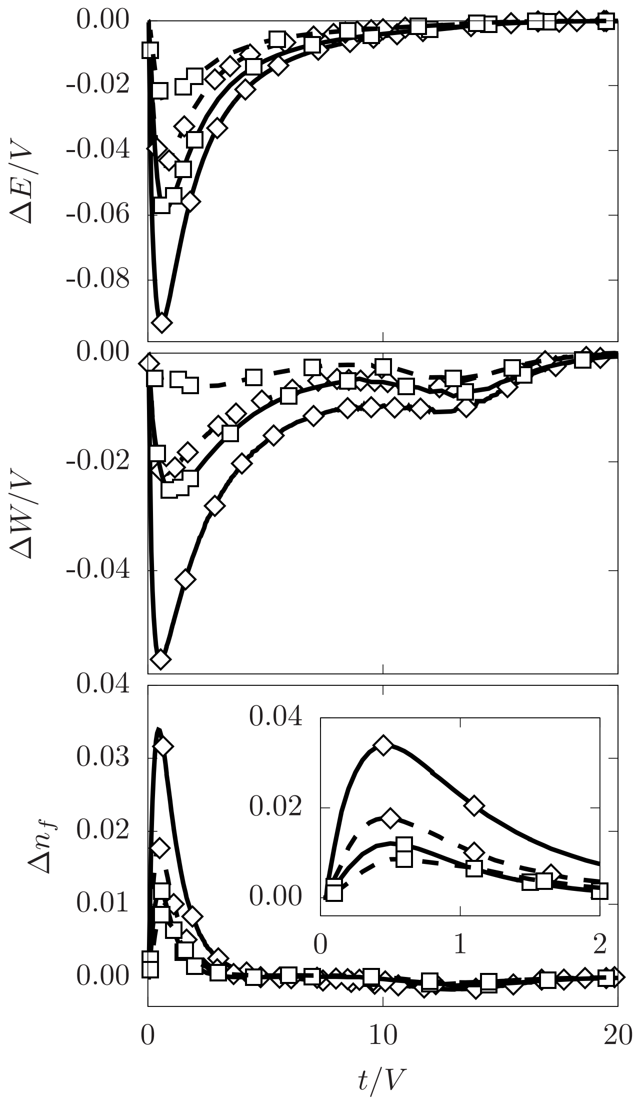


Supplementary Figure S6. Deviation of the ground-state energy $\Delta E = E_{(c)ACA(M)} - E_{\text{exact}}$, interaction energy $\Delta W = W_{(c)ACA(M)} - W_{\text{exact}}$ and impurity occupation $\Delta n_f = n_{f,(c)ACA(M)} - n_{f,\text{exact}}$ between the ground state within the (corrected) adaptive cluster approximation and the exact ground state. Same model as in Fig. S4. The corresponding exact results are shown in Fig. S4. Solid lines correspond to the uncorrected ACA and dashed lines to the Müller-corrected ACA results. Truncation with $M = 1$ (solid line with diamonds) and $M = 2$ (solid line with squares). The results for $M = 3$ are not shown, because they agree with the exact results within the convergence criteria.
